# Supplementary material for: Dual Geometric Graph Network (DG2N) -- Iterative network for deformable shape alignment
Source: arXiv:2011.14723 source file (2021-03-27)
Supplement: Supplementary file 1 [file supplementary.tex]

\newpage
\newpage
\section{Supplementary}

\subsection{Architecture details}
\subsubsection{NaiveNet}
In tables \ref{tab:dgcnnblock}, \ref{tab:NaiveNet_architecture} we provide specific network configurations to construct NaiveNet. Each input shape $\source$ is being transformed by random augmentations woth the parameters depicted in table \ref{tab:NaiveNet_augmentations} resulting in $\grave{\source}$. Both shapes enter into a Siamese structure of NaiveNet resulting in deep features $h_{\source}\in \mathbb{R}^{N\times F},h_{\grave{\source}}\in \mathbb{R}^{N\times F}$. Using the deep features we compute $\softP$ according the cosine-similarity between the features and evaluate the self-supervised loss of NaiveNet \ref{eq:naivenetloss}.
\begin{table}[h]
\begin{tabular}{clll}
Step                   & \multicolumn{1}{c}{Layer} & \multicolumn{1}{c}{Input size} & \multicolumn{1}{c}{Output size} \\ \hline
\multicolumn{1}{c|}{1} & Neighbor pooling          & BxNxI                          & BxNxKxI                         \\
\multicolumn{1}{c|}{2} & Conv 2D 1x1               & BxNxKxI                        & BxNxKxO                         \\
\multicolumn{1}{c|}{3} & BatchNorm 2D              & BxNxKxO                        & BxNxKxO                         \\
\multicolumn{1}{c|}{4} & LeakyRelu                 & BxNxKxO                        & BxNxKxO                         \\
\multicolumn{1}{c|}{5} & NeighborMax               & BxNxKxO                        & BxNxKxO                        
\end{tabular}
\caption{DGCNN block, I,O are the Input/Output feature vectors dimensions.}
\label{tab:dgcnnblock}
\end{table}

\begin{table}[h]
\begin{tabular}{cccc}
\multicolumn{1}{l}{Step} & Layer & \multicolumn{1}{l}{Input size} & \multicolumn{1}{l}{Output size} \\ \hline
\multicolumn{1}{c|}{1}   & DGCNN block               & 3                              & 64                              \\
\multicolumn{1}{c|}{2}   & DGCNN block               & 64                             & 128                             \\
\multicolumn{1}{c|}{3}   & DGCNN block               & 128                            & 256                             \\
\multicolumn{1}{c|}{4}   & DGCNN block               & 256                            & 512                             \\
\multicolumn{1}{c|}{5}   & Concatenate (1,2,3,4)     & *                              & 960                             \\
\multicolumn{1}{c|}{6}   & Linear layer              & 960                            & 512                             \\
\multicolumn{1}{c|}{7}   & BatchNorm1D               & 512                            & 512                            
\end{tabular}
\caption{NaiveNet architecture parameters.}
\label{tab:NaiveNet_architecture}
\end{table}

\begin{table}[h]
\resizebox{\textwidth}{!}{%
\begin{tabular}{ccc}
Augmentation                           & Value      & \# Parameters per shape \\ \hline
Rotation X,Y,Z (degrees)               & -180 - 180        & 3 (per axis)            \\
Scale (multiplicative)                 & 0.2-5             & 1 (per shape)           \\
Random gaussian noise X,Y,Z (additive) & 0.01* area(shape) & Nx3 (x,y,z per point)  
\end{tabular}%
}
\caption{NaiveNet augmentations. We treat all datasets with the same augmentation parameters.}
\label{tab:NaiveNet_augmentations}
\end{table}

Figure {\color{red}7} provides a visualizations of correspondences generated by NaiveNet. 

NaiveNet is a good choice as an initiator  due to its
modality robustness  (meshes or
points clouds) and stable outcomes on a variety of datasets. Equally important is its superior convergence time compared to all other initiators. See numerical support in table \ref{tab:convergence_times}.

\begin{table}[]
\begin{tabular}{cc}
Architecture                           & Convergence time (Hours) \\ \hline
\multicolumn{1}{c|}{\textbf{NaiveNet}} & \textbf{0.65}            \\
\multicolumn{1}{c|}{FMnet}             & 1.92                     \\
\multicolumn{1}{c|}{SURFMnet}          & 1.93                     \\
\multicolumn{1}{c|}{Cyclic FM}         & 2.11                     \\
\multicolumn{1}{c|}{Unsup FM}          & 2.53                     \\
\multicolumn{1}{c|}{GeoFM}             & 1.66                     \\
\multicolumn{1}{c|}{3Dcoded}           & 4.32                    
\end{tabular}
\caption{Convergence times for different initiators on the FAUST-resampled dataset. NaiveNet is a robust and stable initiator (fair correspondence results as an initial soft correspondence map before DG2N denosing operation), while converging up to 10X times faster than other correspondence methods.}
\label{tab:convergence_times}
\end{table}

\subsubsection{DGAT and DG2N}
In tables \ref{tab:dgat},\ref{tab:dg2n} we specify the different layers and the structure of DGAT, as well as the full pipeline of DG2N. We build DGAT atop  \cite{Fey/Lenssen/2019}, a PyTorch framework designed for geometric NN's.
We perform 4-10 consecutive refinement steps of $DG2N$, where each input  $\softP$ is the output of the previous refinement step.

\begin{table}[!h]
\begin{tabular}{clll}
Step                   & \multicolumn{1}{c}{Layer} & \multicolumn{1}{c}{Input size} & \multicolumn{1}{c}{Output size} \\ \hline
\multicolumn{1}{c|}{1} & Neighbor pooling          & BxNxM                          & BxNxKxM                         \\
\multicolumn{1}{c|}{2} & Difference vector         & BxNxKxM                        & BxNxKx3M                        \\
\multicolumn{1}{c|}{3} & MLP+LN+LR                 & BxNxKx3M                       & BxNxKxM                         \\
\multicolumn{1}{c|}{4} & MLP+LN+LR+MLP             & BxNxKxM                        & BxNxM                          
\end{tabular}
\caption{DGAT block, N,M are in number of vertices in the source,target shapes respectively. LN and LR stands for LayerNorm \cite{layernorm}
 and LeakyRelu respectively}\label{tab:dgat}
\end{table}

\begin{table}[!h]
\begin{tabular}{cccl}
\multicolumn{1}{l}{Step}      & Layer                          & \multicolumn{1}{l}{Topology} & Output                          \\ \hline
\multicolumn{1}{c|}{1.source} & DGAT block x 3                 & Source                       & $\softP\in \mathbb{R}^{N\times M}$                    \\
\multicolumn{1}{c|}{1.target} & DGAT block x 3                 & Target                       & $\softP_t\in \mathbb{R}^{M\times N}$ \\
\multicolumn{1}{c|}{2}        & $P_t = P_t^T$ & -                            & $\softP_t\in \mathbb{R}^{N\times M}$                       \\
\multicolumn{1}{c|}{3}        & $\tilde{P} = \frac{P_s + P_t}{2}$      & -                            & $\softP\in \mathbb{R}^{N\times M}$                   
\end{tabular}
\caption{DG2N block, we apply 3 DGAT layers on each soft correspondence mapping ($\softP,\softP^T$) followed by a fusion of the refined statistics.}
\label{tab:dg2n}
\end{table}

\subsection{ablation}
In addition to the numerical evaluation of the importance of the different objectives, we include a visual example of the effect of disabling the anchor guidance in figure {\color{red}8}.
\begin{center}
\begin{table*}

    \begin{tabular}{cccc}
    \noalign{\smallskip}
      SMAL &
    \adjustimage{width=.30\textwidth,valign=c}{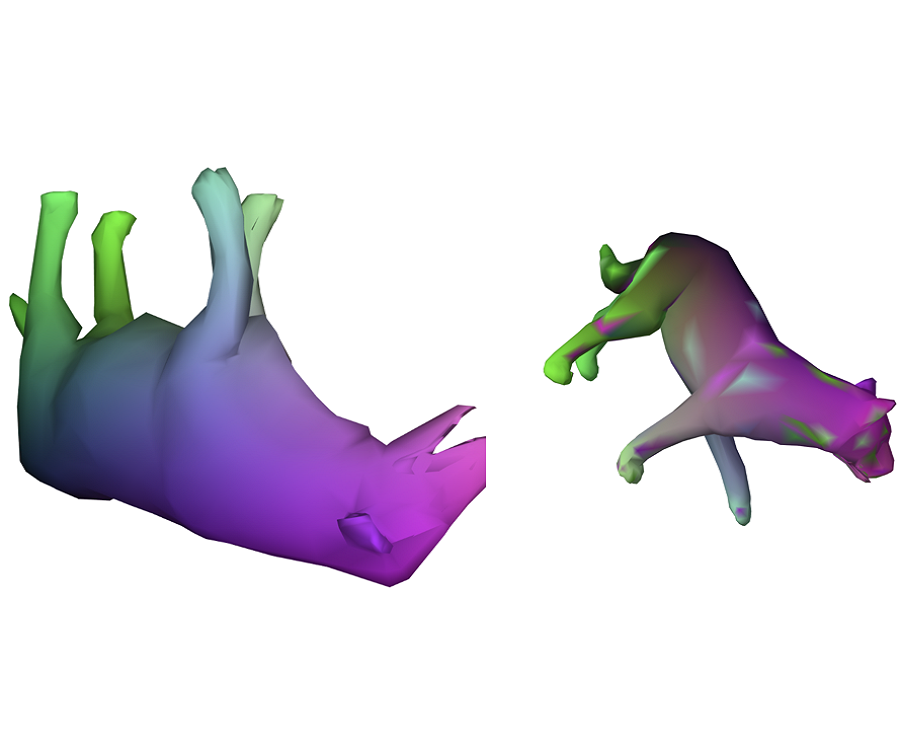}&
    \adjustimage{width=.30\textwidth,valign=c}{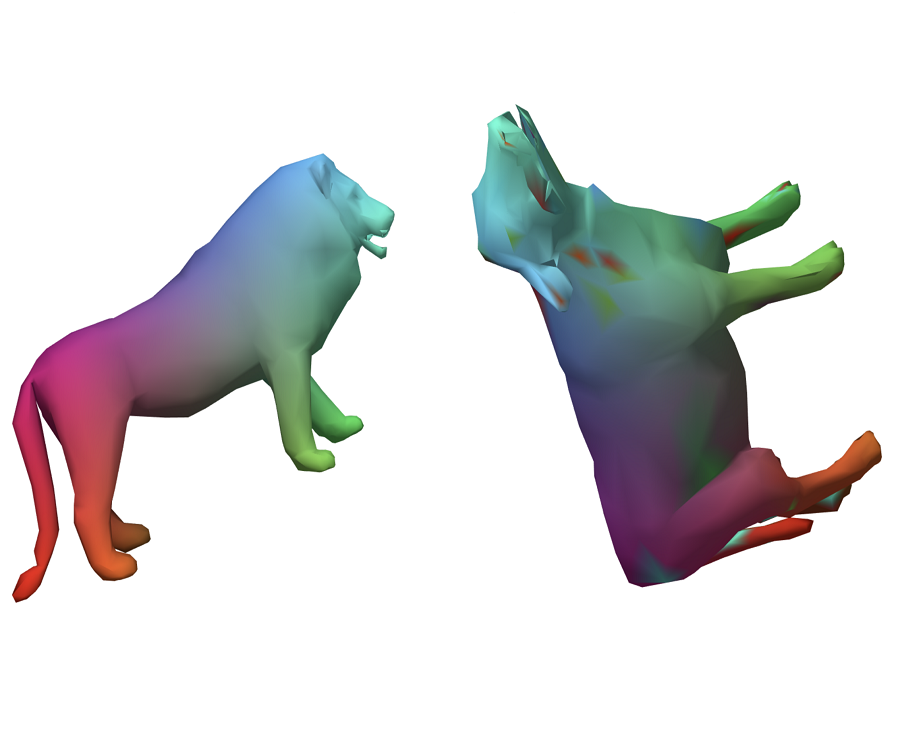}&
    \adjustimage{width=.30\textwidth,valign=c}{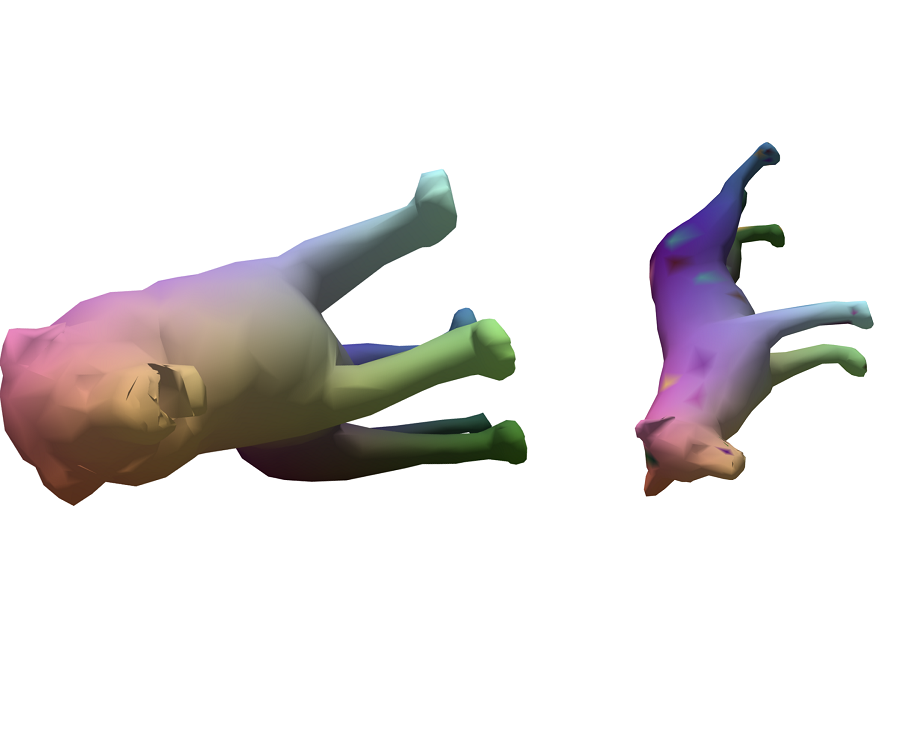}\\
    \noalign{\smallskip}
    FAUST &
    \adjustimage{width=.30\textwidth,valign=c}{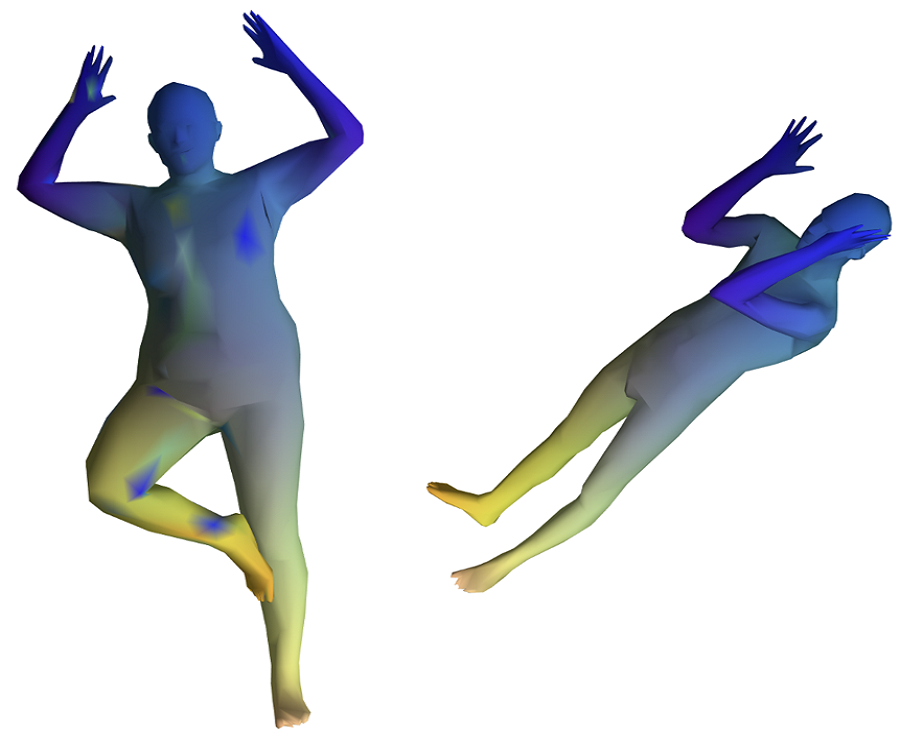}&
    \adjustimage{width=.30\textwidth,valign=c}{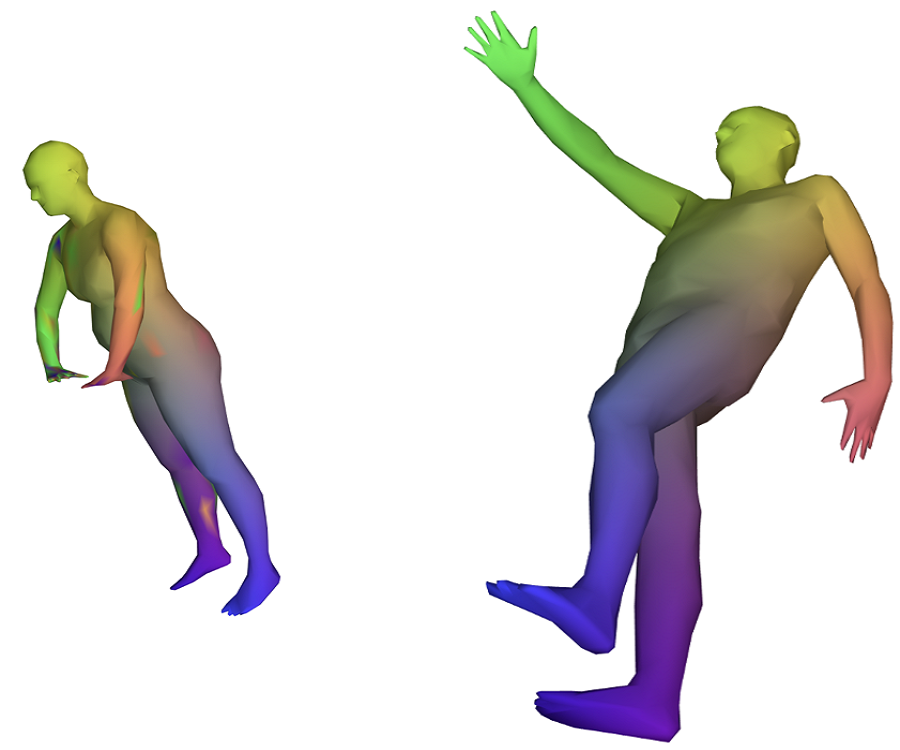}&
    \adjustimage{width=.30\textwidth,valign=c}{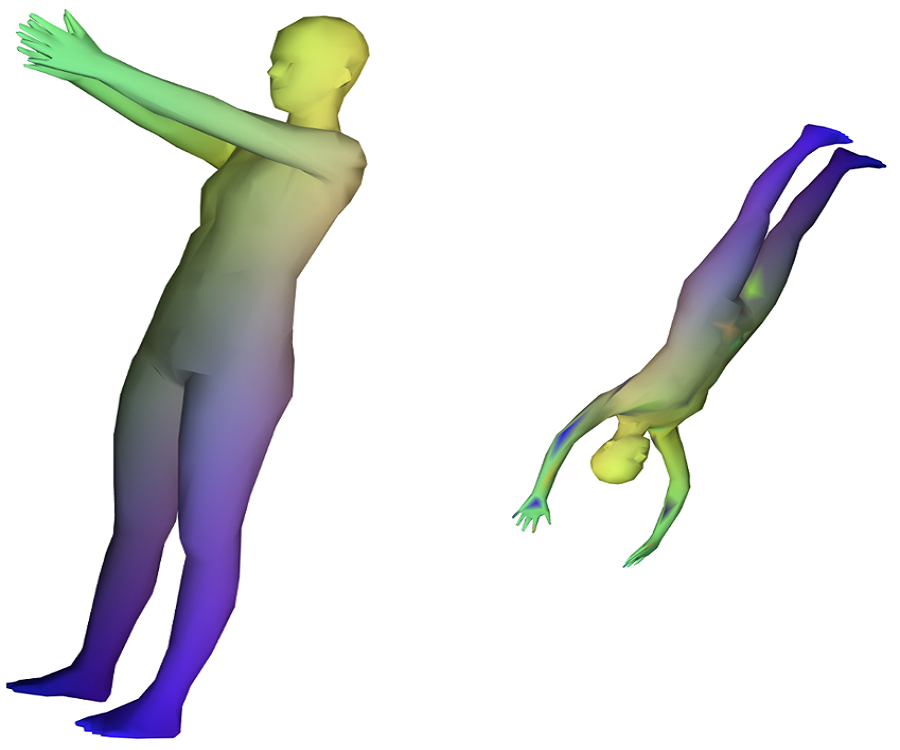}\\
    
    \end{tabular}
      \caption*{\textbf{Figure 7}: Naivenet correspondence examples, the network was only trained on same-shape different-augmentations pairs, resulting with reasonable correspondences even for non-isometric shapes.} \label{fig:naivenet_corr}
\end{table*}
\end{center}

\begin{center}
\begin{table*}[btp]
    \begin{tabular}{ccccccc}
    \noalign{\smallskip}
      No $\mathcal{L}_{AG}$ &
    \adjustimage{width=.10\textwidth,valign=c}{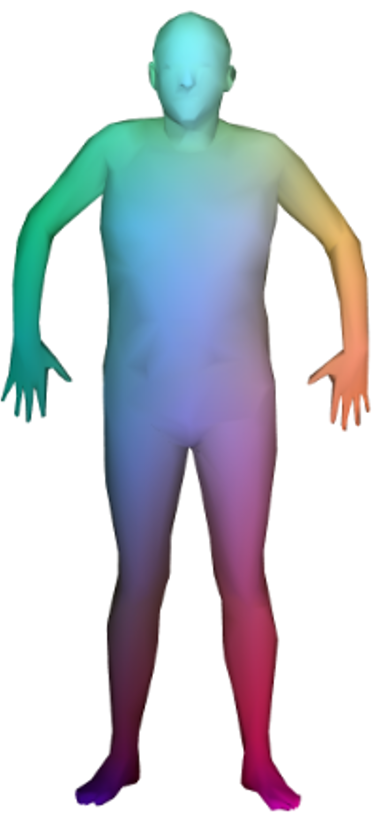}&
    \adjustimage{width=.10\textwidth,valign=c}{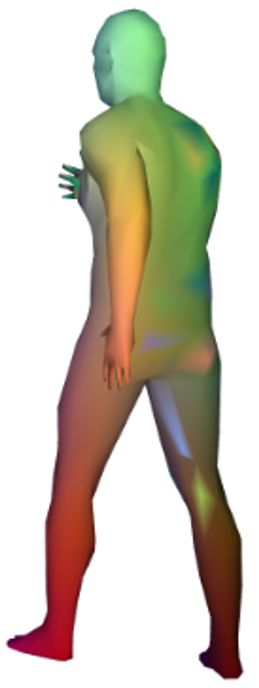}&
    \adjustimage{width=.10\textwidth,valign=c}{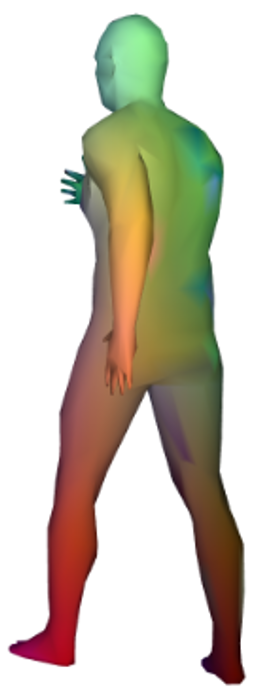}&
    \adjustimage{width=.10\textwidth,valign=c}{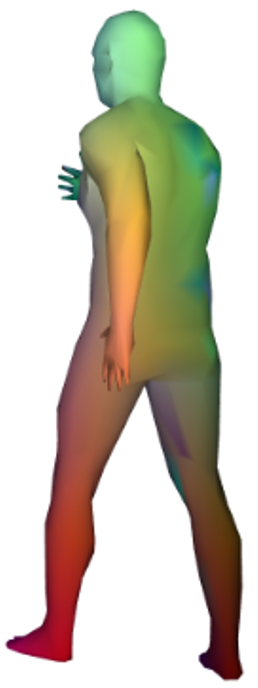}&
    \adjustimage{width=.10\textwidth,valign=c}{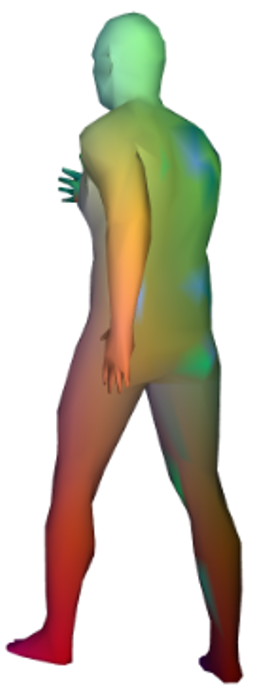}&
    \adjustimage{width=.10\textwidth,valign=c}{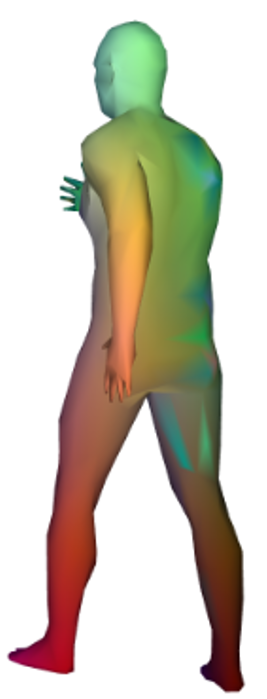}\\
    \noalign{\smallskip}
     With $\mathcal{L}_{AG}$ &
    \adjustimage{width=.10\textwidth,valign=c}{Sections/supplementary/images/ag/reference.PNG}&
    \adjustimage{width=.10\textwidth,valign=c}{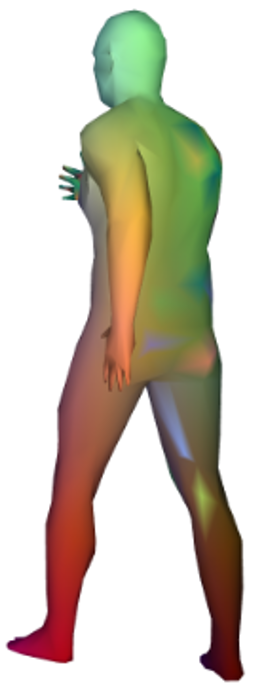}&
    \adjustimage{width=.10\textwidth,valign=c}{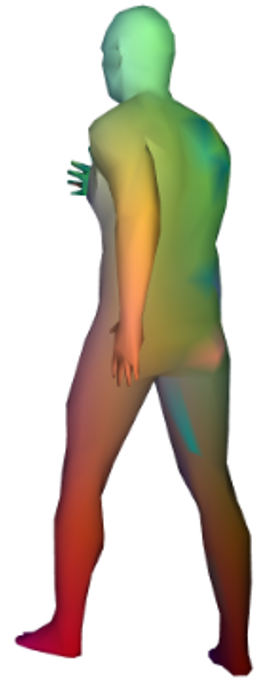}&
    \adjustimage{width=.10\textwidth,valign=c}{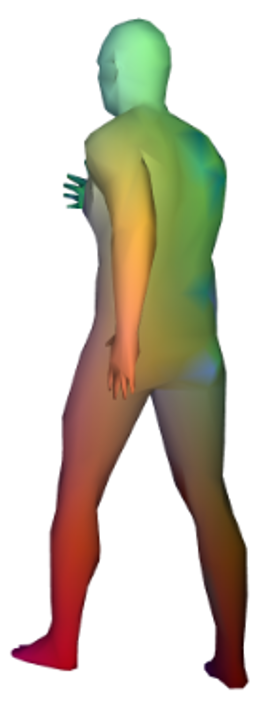}&
    \adjustimage{width=.10\textwidth,valign=c}{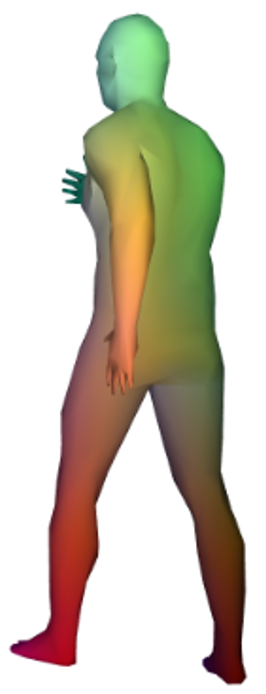}&
    \adjustimage{width=.10\textwidth,valign=c}{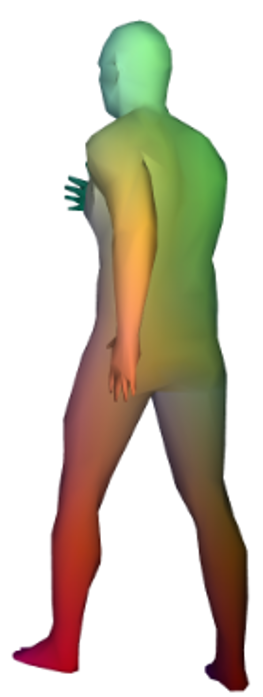}\\
    \noalign{\smallskip}
    \ &
    NaiveNet&
    Step 1&
    Step 2&
    Step 3&
    Step 4&
    Step 5\\
    
    \end{tabular}
\caption*{\textbf{Figure 8}: Correspondence refinement without and with $\mathcal{L}_{AG}$. Without the anchor guidance mechanism the iterative refinment "forgets" the initial correspondences that had high probability by the initiator, resulting in degregation in the results within several steps of the refinment.}
  \label{fig:anchor_guidence}
\end{table*}
\end{center}
