# Supplementary material for: Dual Geometric Graph Network (DG2N) -- Iterative network for deformable shape alignment
Source: arXiv:2011.14723 source file (2021-03-27)
Supplement: Supplementary file 2 [file ablation.tex]

\subsection{ablation}
In addition to the numerical evaluation of the importance of the different objectives, we include a visual example of the effect of disabling the anchor guidance in figure {\color{red}8}.
\begin{center}
\begin{table*}

    \begin{tabular}{cccc}
    \noalign{\smallskip}
      SMAL &
    \adjustimage{width=.30\textwidth,valign=c}{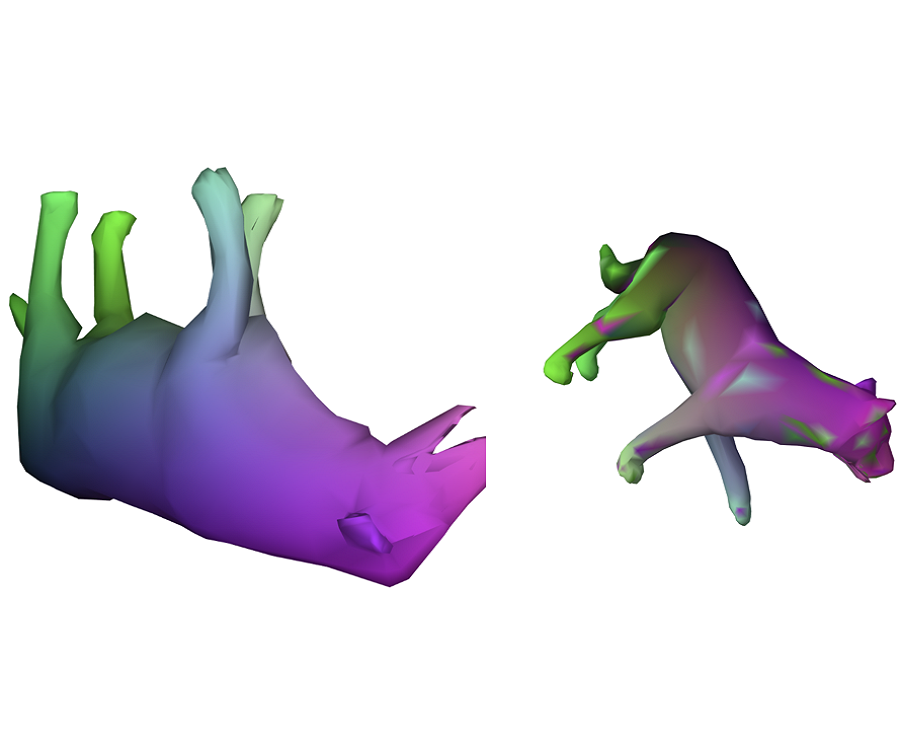}&
    \adjustimage{width=.30\textwidth,valign=c}{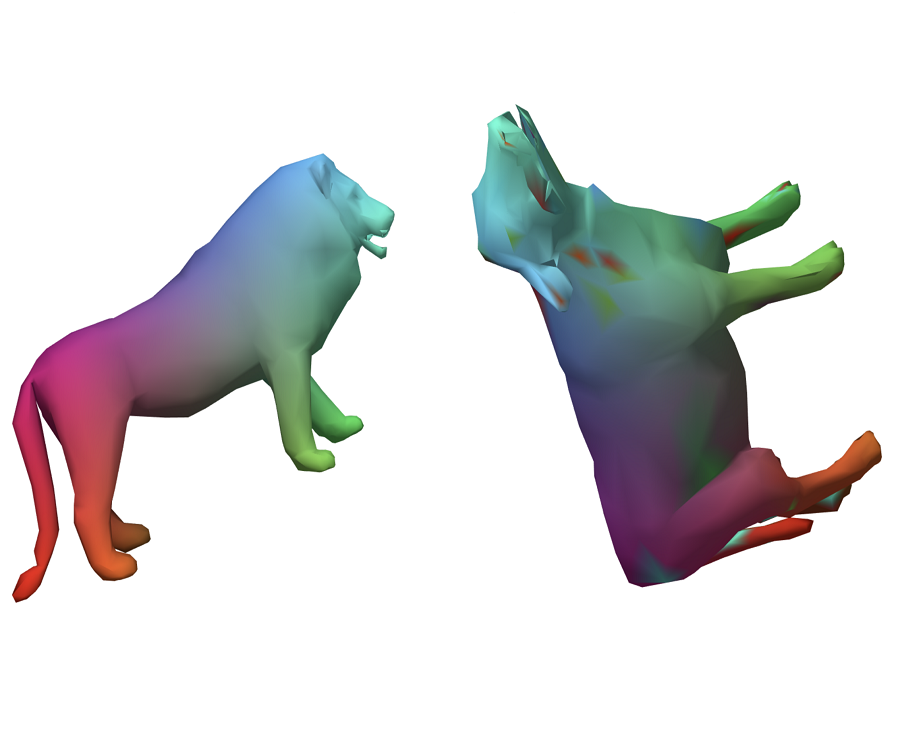}&
    \adjustimage{width=.30\textwidth,valign=c}{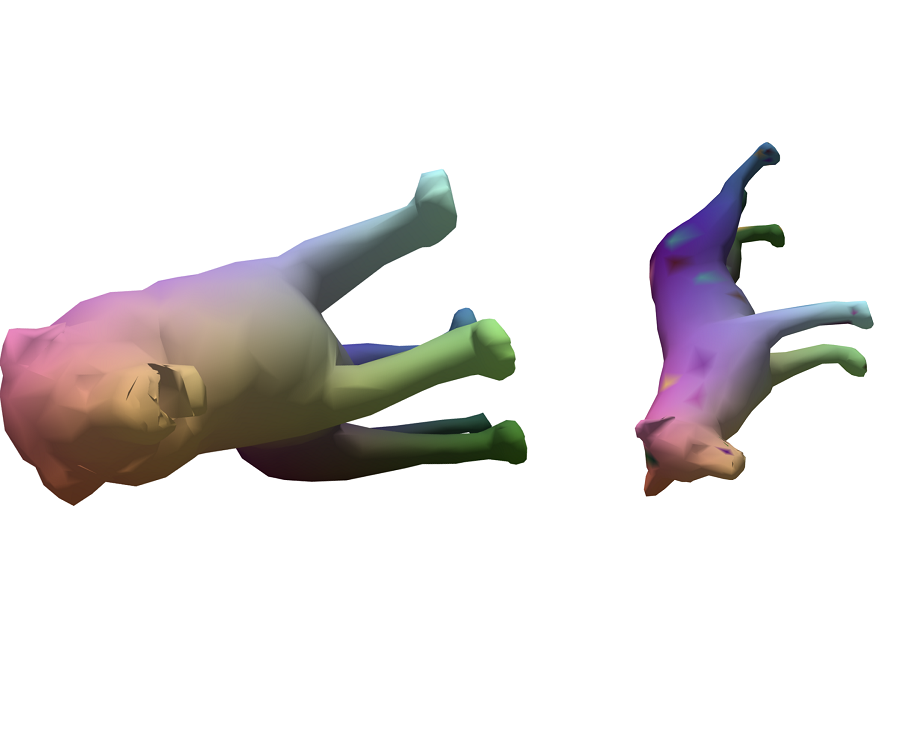}\\
    \noalign{\smallskip}
    FAUST &
    \adjustimage{width=.30\textwidth,valign=c}{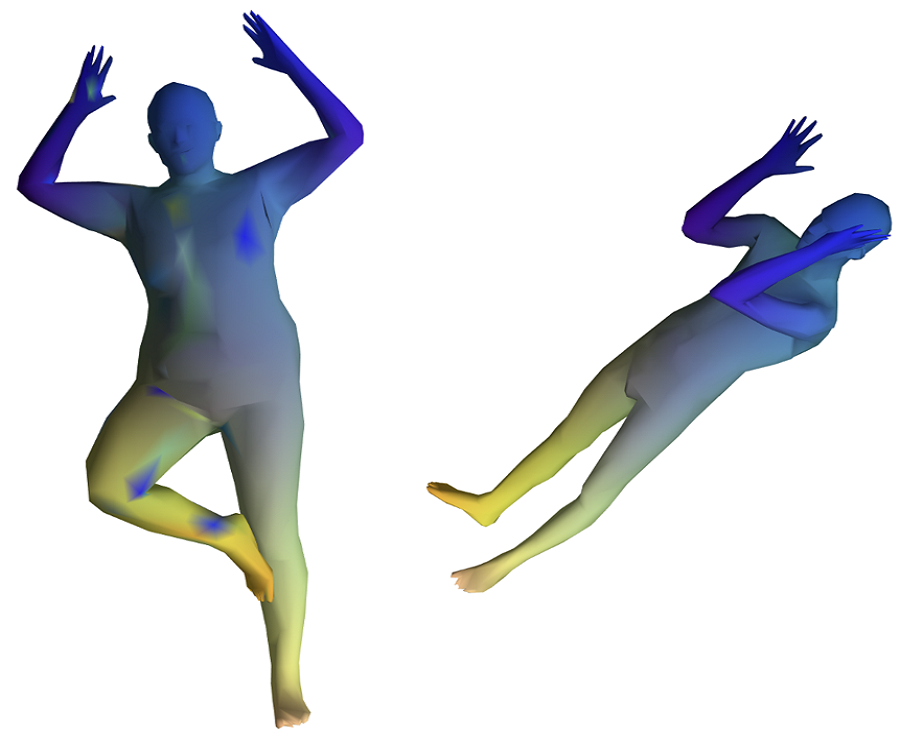}&
    \adjustimage{width=.30\textwidth,valign=c}{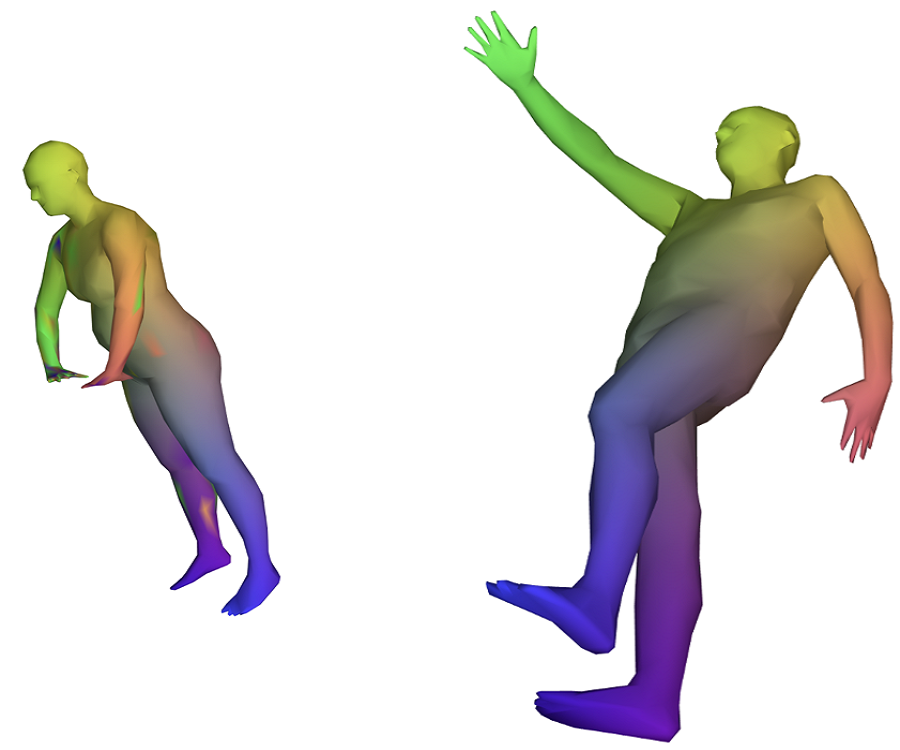}&
    \adjustimage{width=.30\textwidth,valign=c}{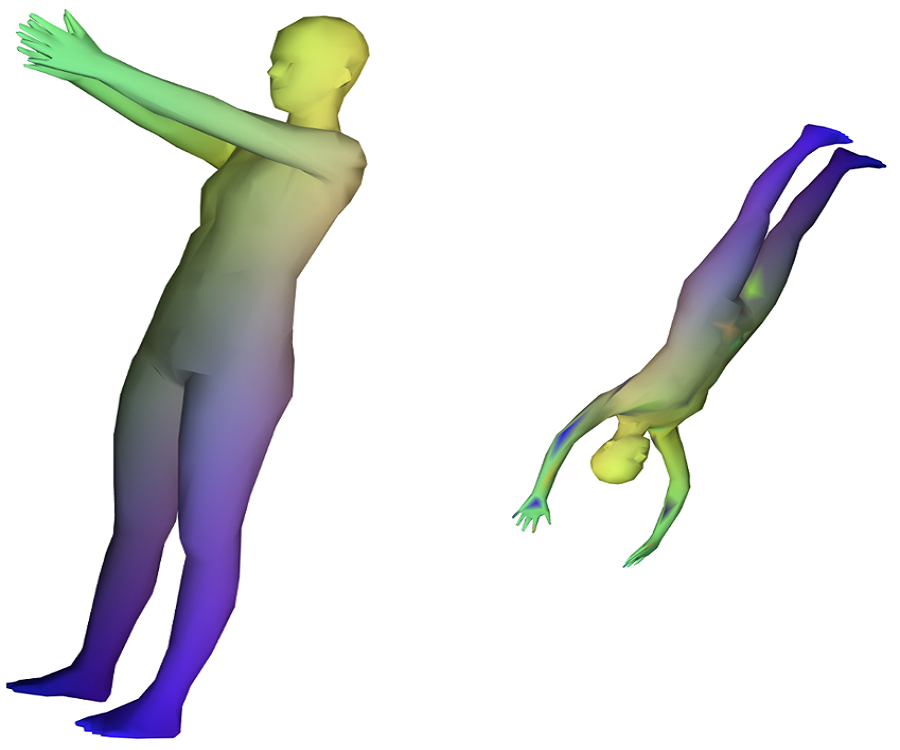}\\
    
    \end{tabular}
      \caption*{\textbf{Figure 7}: Naivenet correspondence examples, the network was only trained on same-shape different-augmentations pairs, resulting with reasonable correspondences even for non-isometric shapes.} \label{fig:naivenet_corr}
\end{table*}
\end{center}

\begin{center}
\begin{table*}[btp]
    \begin{tabular}{ccccccc}
    \noalign{\smallskip}
      No $\mathcal{L}_{AG}$ &
    \adjustimage{width=.10\textwidth,valign=c}{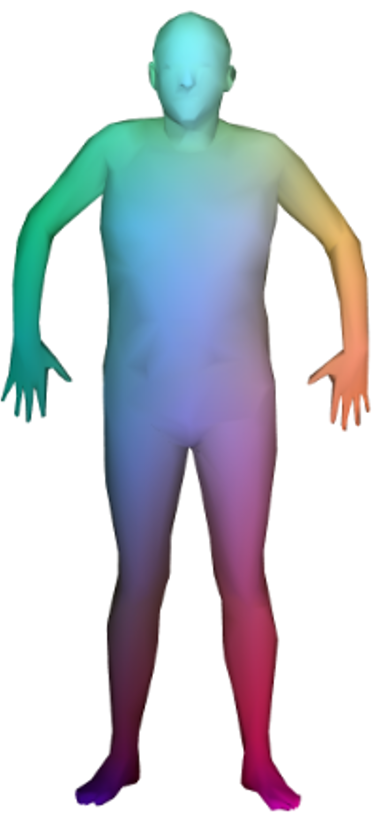}&
    \adjustimage{width=.10\textwidth,valign=c}{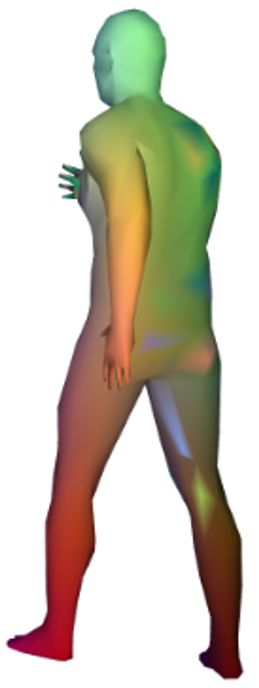}&
    \adjustimage{width=.10\textwidth,valign=c}{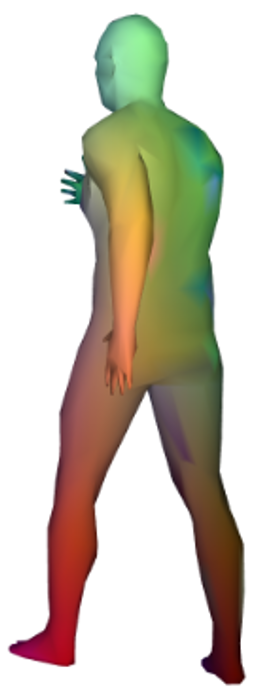}&
    \adjustimage{width=.10\textwidth,valign=c}{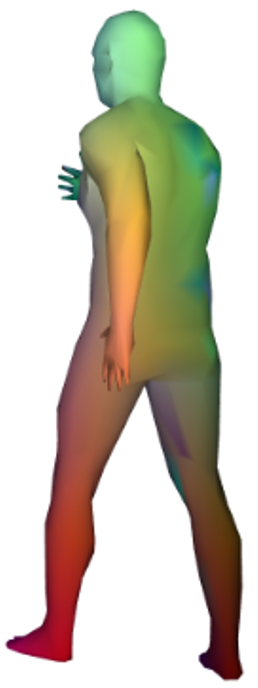}&
    \adjustimage{width=.10\textwidth,valign=c}{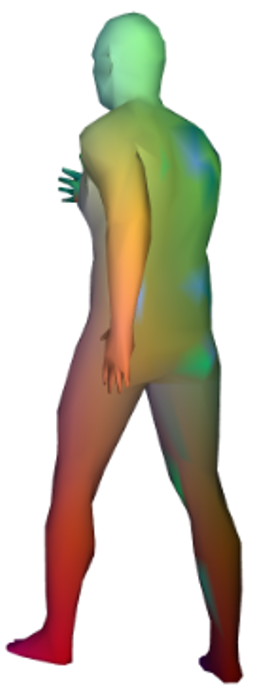}&
    \adjustimage{width=.10\textwidth,valign=c}{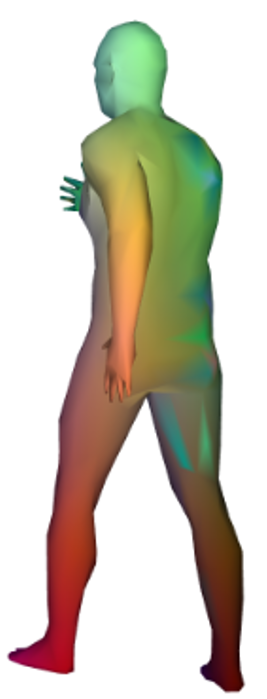}\\
    \noalign{\smallskip}
     With $\mathcal{L}_{AG}$ &
    \adjustimage{width=.10\textwidth,valign=c}{Sections/supplementary/images/ag/reference.PNG}&
    \adjustimage{width=.10\textwidth,valign=c}{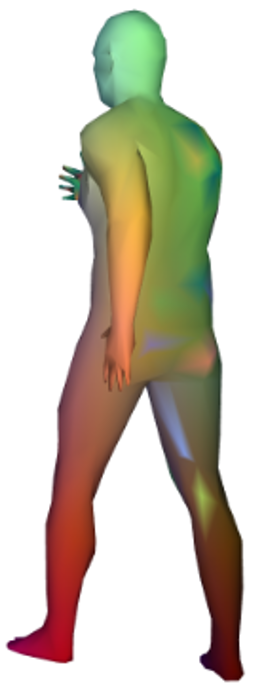}&
    \adjustimage{width=.10\textwidth,valign=c}{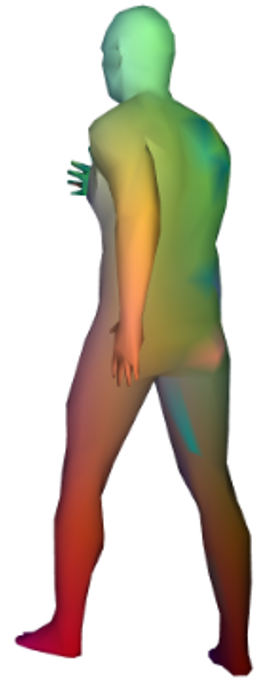}&
    \adjustimage{width=.10\textwidth,valign=c}{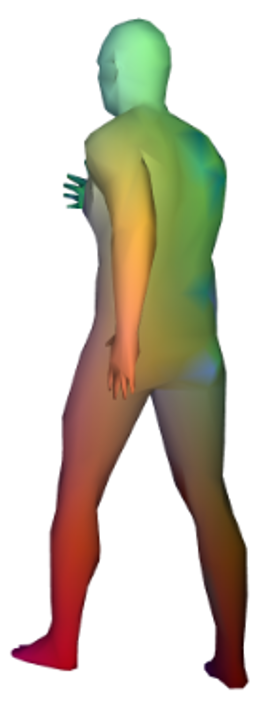}&
    \adjustimage{width=.10\textwidth,valign=c}{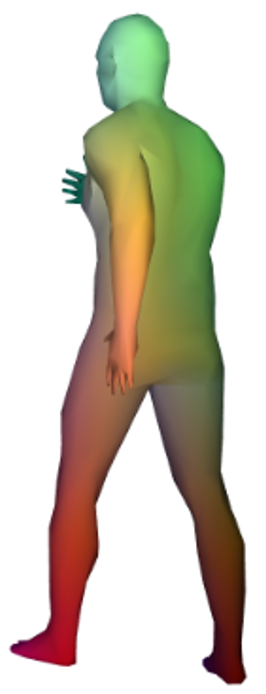}&
    \adjustimage{width=.10\textwidth,valign=c}{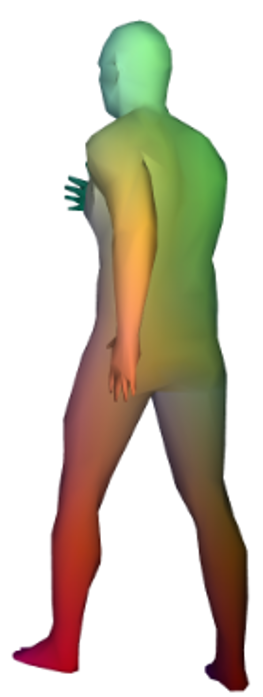}\\
    \noalign{\smallskip}
    \ &
    NaiveNet&
    Step 1&
    Step 2&
    Step 3&
    Step 4&
    Step 5\\
    
    \end{tabular}
\caption*{\textbf{Figure 8}: Correspondence refinement without and with $\mathcal{L}_{AG}$. Without the anchor guidance mechanism the iterative refinment "forgets" the initial correspondences that had high probability by the initiator, resulting in degregation in the results within several steps of the refinment.}
  \label{fig:anchor_guidence}
\end{table*}
\end{center}
