# Supplementary material for: Dual Geometric Graph Network (DG2N) -- Iterative network for deformable shape alignment
Source: arXiv:2011.14723 source file (2021-03-27)
Supplement: Supplementary file 3 [file dgat.tex]

\subsubsection{DGAT and DG2N}
In tables \ref{tab:dgat},\ref{tab:dg2n} we specify the different layers and the structure of DGAT, as well as the full pipeline of DG2N. We build DGAT atop  \cite{Fey/Lenssen/2019}, a PyTorch framework designed for geometric NN's.
We perform 4-10 consecutive refinement steps of $DG2N$, where each input  $\softP$ is the output of the previous refinement step.

\begin{table}[!h]
\begin{tabular}{clll}
Step                   & \multicolumn{1}{c}{Layer} & \multicolumn{1}{c}{Input size} & \multicolumn{1}{c}{Output size} \\ \hline
\multicolumn{1}{c|}{1} & Neighbor pooling          & BxNxM                          & BxNxKxM                         \\
\multicolumn{1}{c|}{2} & Difference vector         & BxNxKxM                        & BxNxKx3M                        \\
\multicolumn{1}{c|}{3} & MLP+LN+LR                 & BxNxKx3M                       & BxNxKxM                         \\
\multicolumn{1}{c|}{4} & MLP+LN+LR+MLP             & BxNxKxM                        & BxNxM                          
\end{tabular}
\caption{DGAT block, N,M are in number of vertices in the source,target shapes respectively. LN and LR stands for LayerNorm \cite{layernorm}
 and LeakyRelu respectively}\label{tab:dgat}
\end{table}

\begin{table}[!h]
\begin{tabular}{cccl}
\multicolumn{1}{l}{Step}      & Layer                          & \multicolumn{1}{l}{Topology} & Output                          \\ \hline
\multicolumn{1}{c|}{1.source} & DGAT block x 3                 & Source                       & $\softP\in \mathbb{R}^{N\times M}$                    \\
\multicolumn{1}{c|}{1.target} & DGAT block x 3                 & Target                       & $\softP_t\in \mathbb{R}^{M\times N}$ \\
\multicolumn{1}{c|}{2}        & $P_t = P_t^T$ & -                            & $\softP_t\in \mathbb{R}^{N\times M}$                       \\
\multicolumn{1}{c|}{3}        & $\tilde{P} = \frac{P_s + P_t}{2}$      & -                            & $\softP\in \mathbb{R}^{N\times M}$                   
\end{tabular}
\caption{DG2N block, we apply 3 DGAT layers on each soft correspondence mapping ($\softP,\softP^T$) followed by a fusion of the refined statistics.}
\label{tab:dg2n}
\end{table}
