# Supplementary material for: Dual Geometric Graph Network (DG2N) -- Iterative network for deformable shape alignment
Source: arXiv:2011.14723 source file (2021-03-27)
Supplement: Supplementary file 4 [file implementation.tex]

\subsection{Architecture details}
\subsubsection{NaiveNet}
In tables \ref{tab:dgcnnblock}, \ref{tab:NaiveNet_architecture} we provide specific network configurations to construct NaiveNet. Each input shape $\source$ is being transformed by random augmentations woth the parameters depicted in table \ref{tab:NaiveNet_augmentations} resulting in $\grave{\source}$. Both shapes enter into a Siamese structure of NaiveNet resulting in deep features $h_{\source}\in \mathbb{R}^{N\times F},h_{\grave{\source}}\in \mathbb{R}^{N\times F}$. Using the deep features we compute $\softP$ according the cosine-similarity between the features and evaluate the self-supervised loss of NaiveNet \ref{eq:naivenetloss}.
\begin{table}[h]
\begin{tabular}{clll}
Step                   & \multicolumn{1}{c}{Layer} & \multicolumn{1}{c}{Input size} & \multicolumn{1}{c}{Output size} \\ \hline
\multicolumn{1}{c|}{1} & Neighbor pooling          & BxNxI                          & BxNxKxI                         \\
\multicolumn{1}{c|}{2} & Conv 2D 1x1               & BxNxKxI                        & BxNxKxO                         \\
\multicolumn{1}{c|}{3} & BatchNorm 2D              & BxNxKxO                        & BxNxKxO                         \\
\multicolumn{1}{c|}{4} & LeakyRelu                 & BxNxKxO                        & BxNxKxO                         \\
\multicolumn{1}{c|}{5} & NeighborMax               & BxNxKxO                        & BxNxKxO                        
\end{tabular}
\caption{DGCNN block, I,O are the Input/Output feature vectors dimensions.}
\label{tab:dgcnnblock}
\end{table}

\begin{table}[h]
\begin{tabular}{cccc}
\multicolumn{1}{l}{Step} & Layer & \multicolumn{1}{l}{Input size} & \multicolumn{1}{l}{Output size} \\ \hline
\multicolumn{1}{c|}{1}   & DGCNN block               & 3                              & 64                              \\
\multicolumn{1}{c|}{2}   & DGCNN block               & 64                             & 128                             \\
\multicolumn{1}{c|}{3}   & DGCNN block               & 128                            & 256                             \\
\multicolumn{1}{c|}{4}   & DGCNN block               & 256                            & 512                             \\
\multicolumn{1}{c|}{5}   & Concatenate (1,2,3,4)     & *                              & 960                             \\
\multicolumn{1}{c|}{6}   & Linear layer              & 960                            & 512                             \\
\multicolumn{1}{c|}{7}   & BatchNorm1D               & 512                            & 512                            
\end{tabular}
\caption{NaiveNet architecture parameters.}
\label{tab:NaiveNet_architecture}
\end{table}

\begin{table}[h]
\resizebox{\textwidth}{!}{%
\begin{tabular}{ccc}
Augmentation                           & Value      & \# Parameters per shape \\ \hline
Rotation X,Y,Z (degrees)               & -180 - 180        & 3 (per axis)            \\
Scale (multiplicative)                 & 0.2-5             & 1 (per shape)           \\
Random gaussian noise X,Y,Z (additive) & 0.01* area(shape) & Nx3 (x,y,z per point)  
\end{tabular}%
}
\caption{NaiveNet augmentations. We treat all datasets with the same augmentation parameters.}
\label{tab:NaiveNet_augmentations}
\end{table}

Figure {\color{red}7} provides a visualizations of correspondences generated by NaiveNet. 

NaiveNet is a good choice as an initiator  due to its
modality robustness  (meshes or
points clouds) and stable outcomes on a variety of datasets. Equally important is its superior convergence time compared to all other initiators. See numerical support in table \ref{tab:convergence_times}.

\begin{table}[]
\begin{tabular}{cc}
Architecture                           & Convergence time (Hours) \\ \hline
\multicolumn{1}{c|}{\textbf{NaiveNet}} & \textbf{0.65}            \\
\multicolumn{1}{c|}{FMnet}             & 1.92                     \\
\multicolumn{1}{c|}{SURFMnet}          & 1.93                     \\
\multicolumn{1}{c|}{Cyclic FM}         & 2.11                     \\
\multicolumn{1}{c|}{Unsup FM}          & 2.53                     \\
\multicolumn{1}{c|}{GeoFM}             & 1.66                     \\
\multicolumn{1}{c|}{3Dcoded}           & 4.32                    
\end{tabular}
\caption{Convergence times for different initiators on the FAUST-resampled dataset. NaiveNet is a robust and stable initiator (fair correspondence results as an initial soft correspondence map before DG2N denosing operation), while converging up to 10X times faster than other correspondence methods.}
\label{tab:convergence_times}
\end{table}

\subsubsection{DGAT and DG2N}
In tables \ref{tab:dgat},\ref{tab:dg2n} we specify the different layers and the structure of DGAT, as well as the full pipeline of DG2N. We build DGAT atop  \cite{Fey/Lenssen/2019}, a PyTorch framework designed for geometric NN's.
We perform 4-10 consecutive refinement steps of $DG2N$, where each input  $\softP$ is the output of the previous refinement step.

\begin{table}[!h]
\begin{tabular}{clll}
Step                   & \multicolumn{1}{c}{Layer} & \multicolumn{1}{c}{Input size} & \multicolumn{1}{c}{Output size} \\ \hline
\multicolumn{1}{c|}{1} & Neighbor pooling          & BxNxM                          & BxNxKxM                         \\
\multicolumn{1}{c|}{2} & Difference vector         & BxNxKxM                        & BxNxKx3M                        \\
\multicolumn{1}{c|}{3} & MLP+LN+LR                 & BxNxKx3M                       & BxNxKxM                         \\
\multicolumn{1}{c|}{4} & MLP+LN+LR+MLP             & BxNxKxM                        & BxNxM                          
\end{tabular}
\caption{DGAT block, N,M are in number of vertices in the source,target shapes respectively. LN and LR stands for LayerNorm \cite{layernorm}
 and LeakyRelu respectively}\label{tab:dgat}
\end{table}

\begin{table}[!h]
\begin{tabular}{cccl}
\multicolumn{1}{l}{Step}      & Layer                          & \multicolumn{1}{l}{Topology} & Output                          \\ \hline
\multicolumn{1}{c|}{1.source} & DGAT block x 3                 & Source                       & $\softP\in \mathbb{R}^{N\times M}$                    \\
\multicolumn{1}{c|}{1.target} & DGAT block x 3                 & Target                       & $\softP_t\in \mathbb{R}^{M\times N}$ \\
\multicolumn{1}{c|}{2}        & $P_t = P_t^T$ & -                            & $\softP_t\in \mathbb{R}^{N\times M}$                       \\
\multicolumn{1}{c|}{3}        & $\tilde{P} = \frac{P_s + P_t}{2}$      & -                            & $\softP\in \mathbb{R}^{N\times M}$                   
\end{tabular}
\caption{DG2N block, we apply 3 DGAT layers on each soft correspondence mapping ($\softP,\softP^T$) followed by a fusion of the refined statistics.}
\label{tab:dg2n}
\end{table}
