# Supplementary material for: Dual Geometric Graph Network (DG2N) -- Iterative network for deformable shape alignment
Source: arXiv:2011.14723 source file (2021-03-27)
Supplement: Supplementary file 6 [file results.tex]

\subsection{Results}
\begin{figure}[!h]
\includegraphics[width=1.\linewidth]{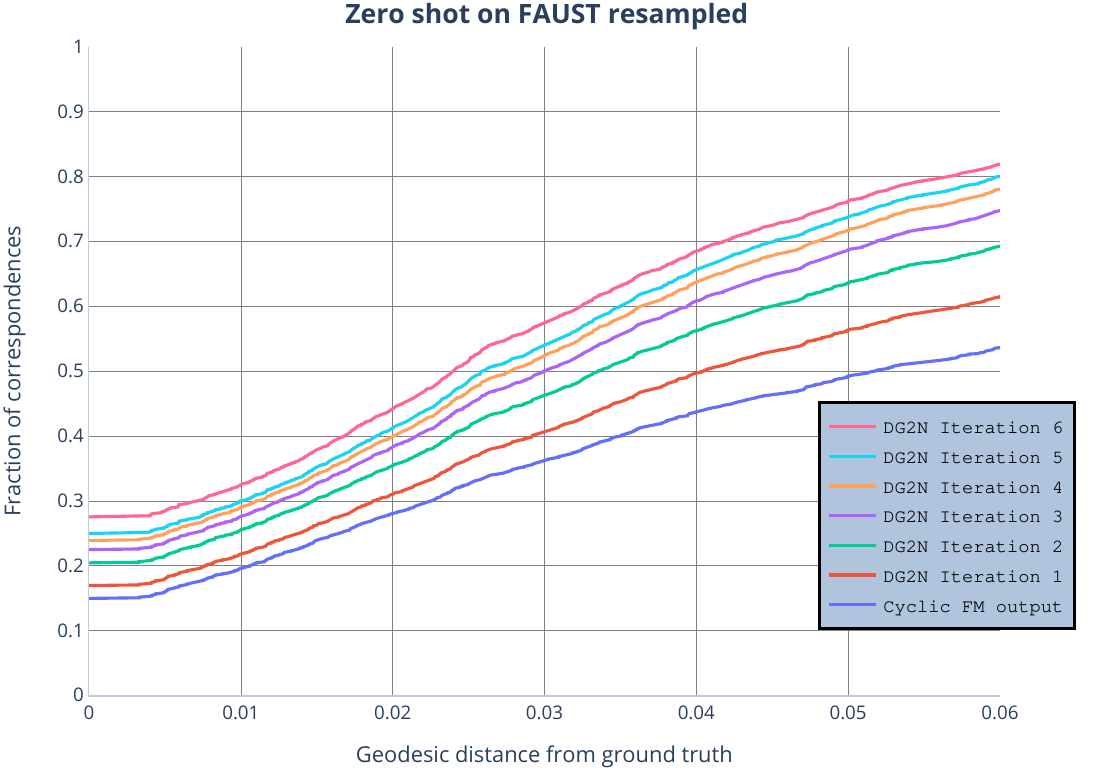}
\caption{Geodesic error on FAUST-remeshed in a self-supervised setting. This figure presents a quantitative evaluation of our network's ability to refine the results in this setting. Both the backbone and DG2N witnessed only augmented versions of the test-pair at training time.}
\label{fig:self_sup_curve}
\end{figure}
