# Supplementary material for: Dual Geometric Graph Network (DG2N) -- Iterative network for deformable shape alignment
Source: arXiv:2011.14723 source file (2021-03-27)

## 6. Supplementary

### 6.1. Architecture details

#### 6.1.1 NaiveNet

In tables 3, 4 we provide specific network configurations to construct NaiveNet. Each input shape  $\mathcal{X}$  is being transformed by random augmentations with the parameters depicted in table 5 resulting in  $\hat{\mathcal{X}}$ . Both shapes enter into a Siamese structure of NaiveNet resulting in deep features  $h_{\mathcal{X}} \in \mathbb{R}^{N \times F}$ ,  $h_{\hat{\mathcal{X}}} \in \mathbb{R}^{N \times F}$ . Using the deep features we compute  $\mathcal{P}$  according the cosine-similarity between the features and evaluate the self-supervised loss of NaiveNet 2.

**Table 3:** DGCNN block, I,O are the Input/Output feature vectors dimensions.

| Step | Layer            | Input size                     | Output size                    |
|------|------------------|--------------------------------|--------------------------------|
| 1    | Neighbor pooling | $B \times N \times I$          | $B \times N \times K \times I$ |
| 2    | Conv 2D 1x1      | $B \times N \times K \times I$ | $B \times N \times K \times O$ |
| 3    | BatchNorm 2D     | $B \times N \times K \times O$ | $B \times N \times K \times O$ |
| 4    | LeakyRelu        | $B \times N \times K \times O$ | $B \times N \times K \times O$ |
| 5    | NeighborMax      | $B \times N \times K \times O$ | $B \times N \times K \times O$ |

**Table 4:** NaiveNet architecture parameters.

| Step | Layer                 | Input size | Output size |
|------|-----------------------|------------|-------------|
| 1    | DGCNN block           | 3          | 64          |
| 2    | DGCNN block           | 64         | 128         |
| 3    | DGCNN block           | 128        | 256         |
| 4    | DGCNN block           | 256        | 512         |
| 5    | Concatenate (1,2,3,4) | *          | 960         |
| 6    | Linear layer          | 960        | 512         |
| 7    | BatchNorm1D           | 512        | 512         |

**Table 5:** NaiveNet augmentations. We treat all datasets with the same augmentation parameters.

| Augmentation                           | Value              | # Parameters per shape |
|----------------------------------------|--------------------|------------------------|
| Rotation X,Y,Z (degrees)               | -180 - 180         | 3 (per axis)           |
| Scale (multiplicative)                 | 0.2-5              | 1 (per shape)          |
| Random gaussian noise X,Y,Z (additive) | 0.01 * area(shape) | Nx3 (x,y,z per point)  |

Figure 7 provides a visualizations of correspondences generated by NaiveNet.

NaiveNet is a good choice as an initiator due to its modality robustness (meshes or points clouds) and stable outcomes on a variety of datasets. Equally important is its superior convergence time compared to all other initiators. See numerical support in table 6.

#### 6.1.2 DGAT and DG2N

In tables 7,8 we specify the different layers and the structure of DGAT, as well as the full pipeline of DG2N. We

**Table 6:** Convergence times for different initiators on the FAUST-resampled dataset. NaiveNet is a robust and stable initiator (fair correspondence results as an initial soft correspondence map before DG2N denosing operation), while converging up to 10X times faster than other correspondence methods.

| Architecture    | Convergence time (Hours) |
|-----------------|--------------------------|
| <b>NaiveNet</b> | <b>0.65</b>              |
| FMnet           | 1.92                     |
| SURFMnet        | 1.93                     |
| Cyclic FM       | 2.11                     |
| Unsup FM        | 2.53                     |
| GeoFM           | 1.66                     |
| 3Dcoded         | 4.32                     |

build DGAT atop [16], a PyTorch framework designed for geometric NN's. We perform 4-10 consecutive refinement steps of  $DG2N$ , where each input  $\mathcal{P}$  is the output of the previous refinement step.

**Table 7:** DGAT block, N,M are in number of vertices in the source,target shapes respectively. LN and LR stands for Layer-Norm [2] and LeakyRelu respectively

| Step | Layer             | Input size                      | Output size                     |
|------|-------------------|---------------------------------|---------------------------------|
| 1    | Neighbor pooling  | $B \times N \times M$           | $B \times N \times K \times M$  |
| 2    | Difference vector | $B \times N \times K \times M$  | $B \times N \times K \times 3M$ |
| 3    | MLP+LN+LR         | $B \times N \times K \times 3M$ | $B \times N \times K \times M$  |
| 4    | MLP+LN+LR+MLP     | $B \times N \times K \times M$  | $B \times N \times M$           |

**Table 8:** DG2N block, we apply 3 DGAT layers on each soft correspondence mapping ( $\mathcal{P}, \mathcal{P}^T$ ) followed by a fusion of the refined statistics.

| Step     | Layer                                                           | Topology | Output                                      |
|----------|-----------------------------------------------------------------|----------|---------------------------------------------|
| 1.source | DGAT block x 3                                                  | Source   | $\mathcal{P} \in \mathbb{R}^{N \times M}$   |
| 1.target | DGAT block x 3                                                  | Target   | $\mathcal{P}_t \in \mathbb{R}^{M \times N}$ |
| 2        | $\mathcal{P}_t = \mathcal{P}_t^T$                               | -        | $\mathcal{P}_t \in \mathbb{R}^{N \times M}$ |
| 3        | $\tilde{\mathcal{P}} = \frac{\mathcal{P}_s + \mathcal{P}_t}{2}$ | -        | $\mathcal{P} \in \mathbb{R}^{N \times M}$   |

## 6.2. Ablation

DG2N training is constructed of 4 different loss functions, each plays an important and substantial rule in the refinement process. We provide table 9 as numerical evidence to the importance of each loss, as well as the effect of disabling combinations of loss functions. The ablation was done on FAUST resampled from the main transcript, with the initial correspondence generated by NaiveNet.

In addition to the numerical evaluation of the importance of the different objectives, we include a visual example of the effect of disabling the anchor guidance in figure 8.

**Table 9:** Ablation study evaluating the significance of the different cost functions. While some objectives improve the refinement effect, some, as  $\mathcal{L}_{AG}$  or  $\mathcal{L}_{l2}$  are indispensable, with substantial degradation to the results without their regularization effect to the denoising process.

| Loss                                                  | MGE        |
|-------------------------------------------------------|------------|
| NaiveNet                                              | 12.2       |
| All                                                   | <b>6.5</b> |
| $\mathcal{L}_L + \mathcal{L}_{l2} + \mathcal{L}_{AG}$ | 8.5        |
| $\mathcal{L}_L + \mathcal{L}_{l1} + \mathcal{L}_{l2}$ | 9.3        |
| $\mathcal{L}_{l2} + \mathcal{L}_{AG}$                 | 12.2       |
| $\mathcal{L}_L + \mathcal{L}_{l1} + \mathcal{L}_{AG}$ | 42.3       |
| $\mathcal{L}_L + \mathcal{L}_{l1}$                    | 55.3       |

**Figure 7:** Naivenet correspondence examples, the network was only trained on same-shape different-augmentations pairs, resulting with reasonable correspondences even for non-isometric shapes.

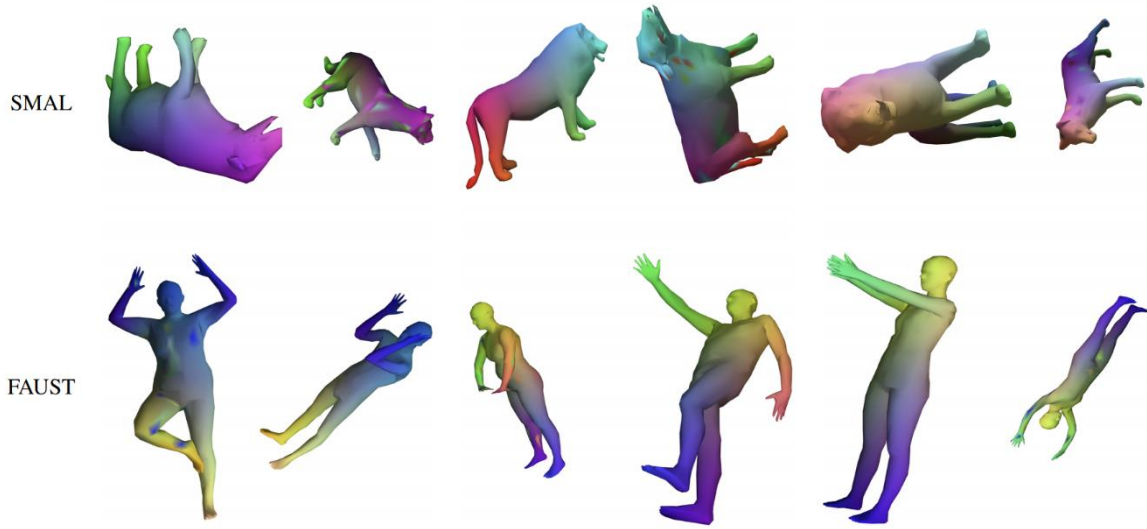

**Figure 8:** Correspondence refinement without and with  $\mathcal{L}_{AG}$ . Without the anchor guidance mechanism the iterative refinement “forgets” the initial correspondences that had high probability by the initiator, resulting in degregation in the results within several steps of the refinement.

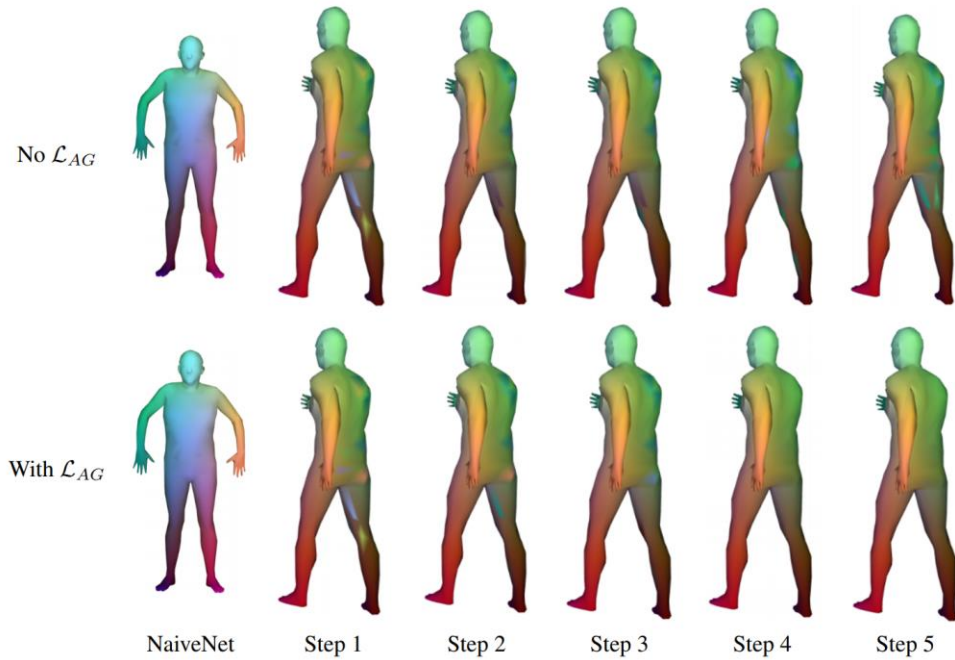

Supplement: Supplementary file 7 [file supp.pdf]
